# Supplementary material for: Solving generalized eigenvalue problems by ordinary differential equations on a quantum computer
Source: arXiv:2010.15027 source file (2021-10-19)
Supplement: Supplementary file 1 [file supplementary.tex]

Let $A$ be a matrix. Let $\lambda$ be a unknown
eigenvalue of $A$, but its eigenvector $|E\rangle$ is known. We want to compute $\lambda$. Consider
the following differential equation.
\be
\begin{cases} \vspace{.2cm}
\ds \frac{d}{dt}|u(t)\rangle = 2\pi iA |u(t)\rangle, \\
u(0) = |E\rangle.
\end{cases}
\ee
Using discretization method, we obtain
\be
\frac{1}{\sqrt{n}} \sum_{j=0}^{n-1} |j\rangle|u(j \Delta t)\rangle
=\frac{1}{\sqrt{n}} \sum_{j=0}^{n-1} e^{2\pi i\lambda j \Delta t}|j\rangle|E\rangle.
\ee
Then apply quantum Fourier inverse transform to the 
first register, we obtain
\be
\frac{1}{n} \sum_{k=0}^{n-1}  \sum_{j=0}^{n-1} e^{2\pi i j (\lambda \Delta t - \frac{k}{n})}|k\rangle|E\rangle \approx
|\lambda \Delta t\rangle|E\rangle.
\ee

Problem 1. Given two real quantum states $|x\rangle,|y\rangle$, we want to compute $\langle x|y\rangle$. 
Typically, we can use swap test or Hadamard test.
Set $A=|x\rangle \langle y|$, then $|x\rangle$ is 
an eigenvector, the corresponding eigenvalue
is $\langle x|y\rangle$.

Problem 2. Matrix multiplication and verification.

This gives a method to solve the
nonlinear eigenvalue problem. 
It suffices to find all the eigenvalues and eigenvectors of the $mn$-by-$mn$ matrix $M$. 
Since all the eigenvectors of this matrix have the form given in (\ref{nonlinear eigenvalue problem:equivalent form}),
all the eigen-pairs are the solutions of
(\ref{nonlinear eigenvalue problem}).
This kind
of method has been investigated in \cite{peters1970ax}.

In the quadratic case, if $A_2,A_1,A_0$ are Hermitian,
then we can find Hermitian linearization:
\be
\left[ \begin{array}{ccccccc}
A_1 & A_0 \\
A_0 & 0   \\
\end{array} \right]
\left[ \begin{array}{ccccccc}
\lambda \x \\
\x   \\
\end{array} \right]
=\lambda \left[ \begin{array}{ccccccc}
-A_2 & 0 \\
0 & A_0   \\
\end{array} \right]
\left[ \begin{array}{ccccccc}
\lambda \x \\
\x   \\
\end{array} \right].
\ee
For cubic eigenvalue problem,
the Hermitian linearization is
\be
\left[ \begin{array}{ccccccc}
A_2 & A_1 & A_0 \\
A_1 & A_0 & 0   \\
A_0 & 0   & 0   \\
\end{array} \right]
\left[ \begin{array}{ccccccc}
\lambda^2 \x \\
\lambda \x \\
\x   \\
\end{array} \right]
=\lambda \left[ \begin{array}{ccccccc}
-A_3 & 0 & 0 \\
0 & A_1 & A_0   \\
0 & A_0 & 0 
\end{array} \right]
\left[ \begin{array}{ccccccc}
\lambda^2 \x \\
\lambda \x \\
\x   \\
\end{array} \right].
\ee
In the general case,

By Euler's method
\be  \label{finite difference 1}
B \frac{d\x(t_l)}{dt} = B \frac{\x(t_{l}) - \x(t_{l-1})}{\Delta t} + O(\|B\|\Delta t).
\ee
So for $l=1,2,\ldots,n-1$, we have
\be \label{finite difference 2}
B \x(t_{l}) - B \x(t_{l-1})  
=\Delta t A\x(t_l)+ O(\|B\|\Delta t^2).
\ee
Set
\be
C = \left[ \begin{array}{ccccccc}
1 \\
-1 & 1 \\
   & \ddots & \ddots \\
   & & -1  & 1
\end{array} \right]_{n\times n}, \quad
\b = \left[ \begin{array}{ccccccc}
B\x(0) \\
0 \\
\vdots \\
0
\end{array} \right]_{n\times 1}
\ee
then we obtain a linear system
\be \label{simple ODE:difference}
(C\otimes B-\Delta t I \otimes A) \widetilde{\x}
= \b.
\ee

\begin{lem}
Let $\x$ be the exact solution of the differential equation (\ref{simple ODE}),
$\widetilde{\x}$ be the exact solution of the
linear system (\ref{simple ODE:difference}),
then
\be
\|\x-\widetilde{\x}\|_2 \leq 
\kappa^3\tau \Delta t^2....
\ee 
where
$\tau = \|B\| \|(B-\Delta t A)^{-1}\|$.
If we choose $p$
\end{lem}

\section{Main idea}

There are at least three methods that
we can investigate to solve the nonlinear
eigenvalue problem.
\begin{enumerate}
\item Use quantum algorithms to solve (\ref{nonlinear eigenvalue problem:equivalent form}).
\item Use quantum differential equation solvers to solve (\ref{ODE}). In this case, there are two possibilities:
\begin{enumerate}
\item Use finite difference method to approximate higher order derivatives, then solve the linear system in a quantum computer.
\item Introduce new variables, change
it into a larger linear system of 
first order differential equations, then use quantum algorithms (e.g. \cite{berry2014high,childs2020quantum,berry2017quantum}) to solve this system of differential equations.
\end{enumerate}
\end{enumerate}

\subsection{Solve the eigenvalue problem (\ref{nonlinear eigenvalue problem:equivalent form})}

This idea is similar to Algorithm 1 of \cite{shao2019computing}. Indeed, we can apply this algorithm directly to solve the eigenvalue problem (\ref{nonlinear eigenvalue problem:equivalent form}).

\begin{thm}[Theorem 2.5 and Corollary 2.8 of \cite{shao2019computing}]
\label{thm1}
Assume that $M$ in (\ref{notation}) is an $s$-sparse diagonalizable matrix which only has real eigenvalues $\{\lambda_1,\ldots,\lambda_{mn}\}$. Assume that the corresponding unit eigenvectors are $\{|E_1\rangle,\ldots,|E_{mn}\rangle\}$. Let $|\lambda_{\max}|$ be a upper bound of the eigenvalues.
Then we can perform the following transformation
\be \label{thm1:transform}
\sum_{j=1}^{mn} \alpha_j |E_j\rangle
\mapsto 
\frac{1}{Z}
\sum_{j=1}^{mn} \alpha_j |\tilde{\lambda}_j\rangle |E_j\rangle
\ee
in time
\be \label{thm1:complexity}
\widetilde{O}(s\kappa^2/\epsilon^2)
\ee
where $Z$ is the normalization factor, $\widetilde{O}$ omits the logarithm terms,
$\kappa$ is the condition number of the matrix generated by 
the eigenvectors and $|\lambda_j-\tilde{\lambda}_j|\leq |\lambda_{\max}|\epsilon$ for all $j$.

\end{thm}

Since $\{|E_1\rangle,\ldots,|E_{mn}\rangle\}$ are linearly independent, any vector of dimension $mn$ is a linear combination of them, which means the left hand side of (\ref{thm1:transform}) can be chosen as any quantum state.
Based on (\ref{notation}), each $|E_j\rangle $ is proportional to $\sum_{k=0}^{m-1} \lambda^k |k\rangle |\x_j\rangle$ 
for some eigenvector $\x_j$ 
of the nonlinear eigenvalue problem (\ref{nonlinear eigenvalue problem}).
So we can rewrite (\ref{thm1:transform}) as
\be 
\sum_{j=1}^{mn} \sum_{k=0}^{m-1}  \alpha_j \lambda^k |k\rangle |\x_j\rangle
\mapsto 
\frac{1}{Z}
\sum_{j=1}^{mn}\sum_{k=0}^{m-1}  \alpha_j\lambda^k |\tilde{\lambda}_j\rangle  |k\rangle |\x_j\rangle
\ee
If $A_i$ has sparsity $s_i$, then the sparsity of $M$ is $\sum_i s_i$, then the complexity becomes $\widetilde{O}(\sum_i s_i\kappa^2/\epsilon^2)$.

Theorem \ref{thm1} needs $A_m$ to be $-I$ or $cI$ for any $c\neq 0$.
In the following we consider the case when $A_m$ is not a multiply of the identity matrix. If $A_m$ is nonsingular, then
(\ref{nonlinear eigenvalue problem}) is 
equivalent to
\be
\lambda^m \x + \sum_{k=0}^{m-1} \lambda^k A_m^{-1}A_k \x = 0.
\ee
Then we can define $M$ by changing $A_i$ into $-A_m^{-1}A_k$. It is also equivalent to
\be
M\widetilde{\x} = \lambda T \widetilde{\x},
\ee
where
\be
T = \left[ \begin{array}{ccccccc}
   I & \\
        & \ddots  \\
        &        & I \\
 &  &   & -A_{m}
\end{array} \right].
\ee
This is a generalized eigenvalue problem.

@article{childs2017lecture,
  title={Lecture notes on quantum algorithms},
  author={Childs, Andrew M},
  year={2017},
  url={https://www.cs.umd.edu/~amchilds/qa/qa.pdf},
}

@article{ashleylecturenote,
  title={Quantum computation - Lecture notes},
  author={Ashley Montanaro},
  url = {https://people.maths.bris.ac.uk/~csxam/partiii/qc-partiii.pdf},
  year={2011}
}
 (see
\cite[Section 1.3]{ashleylecturenote})
